# Supplementary material for: Understanding the LLM-ification of CHI: Unpacking the Impact of LLMs at CHI through a Systematic Literature Review
Source: arXiv:2501.12557 source file (2025-01-22)
Supplement: Supplementary file 1 [file appendix.tex]

\section{Final Codebook}

\begin{table}[H]
\centering
\caption{The final codebook with four code categories as well as the Inter-Rater Reliability. Multiple codes can apply to one paper.}
\begin{tabular}{p{4cm}p{9cm}p{2cm}}
\toprule \midrule
\textbf{Category} & \textbf{Codes} & \textbf{IRR} \\
\midrule 
Contribution Types (7 codes) & Empirical, Artifact, Methodological, Theoretical, Dataset, Metareview, Opinion & \textbf{0.866} \\ \midrule
Application Domain (10 codes) & Communication \& Writing, Augmenting Capabilities, Education, Responsible Computing, Programming, Reliability \& Validity of
LLMs, Well-being \& Health,  Design, Accessibility \& Aging, Creativity & \textbf{0.849} \\ \midrule
Roles of LLMs (5 codes) & LLMs as system engines; LLMs as research tools; LLMs as participants \& users; LLMs as objects of study; Users' perceptions of LLMs  & \textbf{0.773} \\ \midrule
Limitations \& Risks (29 codes) & \textbf{Limitations on LLM Performance} LLM bias toward different groups, limited data coverage in the training data, non-deterministic response, hallucination, unspecificied errors and biases; \textbf{Limitations on Research Validity} internal and/or external validity across users, contexts, models, prompts; \textbf{Limitations on Resource} computational cost, financial cost, lack of evaluation standards; \textbf{Risks to Society, consequences} economic harms, representational harms, misinformation harms, malicious use, hate speech, and environmental harms. &
\textbf{0.887} (\textbf{0.633} for the 29 low-level codes)  \\ 

& \textbf{Note}: \textit{There are 22 low-level codes described in the full paper. However, we had an initial set of 29 low-level code. We had four code ``others'' under each coarse categories (e.g., other LLM performance issues). We also merged three other codes during the coding process (i.e., latency, lack of access to open/close models, prompt-induced performance issues). These codes overlap with the definition of the 22 main codes.}
\\
\midrule

% Non-determinstric reponse; Hallucination; LLM bias toward different groups; Unspecified errors; limits of LLM data coverage; latency; other technical bugs; Internal/External Validity across Users/Contexts/Models/Prompts; Financial Cost; Computational Cost; Open v. Closed models; Proposed modularity without evaluation; Lack of evaluation standards/metrics; Environmental cost; representational harms; privacy; misinformation; malicious use; hate speech & \textbf{0.633}\footnote{\textbf{0.887} for the four coarse-level codes}  \\ \midrule
\bottomrule
\end{tabular}
\end{table}

% Roles of LLMs (5 codes) & (1) LLMs powers the system; (2) LLMs infers user intent; (3) LLMs simulates user behaviors; (4) LLMs improve users’ creativity; (5) LLMs change how users interact with LLMs themselves; (5) study how users use and/or perceive LLMs (systems)  & \textbf{0.773} \\ \midrule

\section{Definition of Contribution Types}

\begin{itemize}
    \item \textbf{Empirical Contribution}: They provide findings based on observation and data-gathering, including experiments, user tests, field observations. Interviews, surveys, focus groups.

    \item \textbf{Artifact Contribution}:  They provide news systems, architectures, tools, toolkits, techniques. 

    \item \textbf{Methodological Contribution}: They inform us how we carry out our work. 
    \begin{itemize}
        \item Note that this contribution type focuses on research methods contribution.
        \item If the paper creates a novel application or framework for users to interact with LLMs (e.g., through prompting or finetuning), it is a methodological contribution.
        \item If the paper uses LLMs to brainstorm in a unique application domains, it is not methodological contribution because they largely rely on the LLMs performance. 
    \end{itemize}

    \item \textbf{Theoretical Contribution}: They consist of new or improved concepts, definitions, models, principles, or frameworks.

    \begin{itemize}
        \item Note that theoretical contributions have to validate or develop theory. 
        \item Drawing from ~\cite{stefanidi2023literature}, if a paper applies or adopts a theory to HCI research, this is a theoretical contribution. 
        \item In other cases the paper's main goal should be developing a theory (e.g., design theory, ethical theory, guideline, framework, design space).
        \item If a paper comes up with design requirement as a formative study or in the discussion section or design implications section, they are not theoretical contribution. 
    \end{itemize}

    \item \textbf{Dataset Contribution}: They provide a new and useful corpus, often accompanied by an analysis of its characteristics, for the benefit of the research community. Note that we only count dataset contribution if the paper open sources the data, or explicitly mention the contribution type.

    \item \textbf{Survey/Metareview Contribution}: Survey research contributions and 
other meta-analyses review and 
synthesize work done on a research 
topic with the goal of exposing trends 
and gaps

    \item \textbf{Opinion Contribution}: Opinion research contributions, also  called essays or arguments, seek to change the minds of readers through persuasion. They are position papers. Note that every paper might convey some opinions, but the major contribution should be considered. 
    
\end{itemize}
